# Supplementary material for: WayTrace: A Map-to-Language-to-Trace Hierarchy for Embodied Urban Navigation
Source: arXiv:2611.05129 source file (2026-11-03)
Supplement: Supplementary file 1 [file supp_failures.tex]

CityWalker & 0 & 30 & \textcolor{black!35}{0} & \textcolor{black!35}{0} & 2 & 4 & \textcolor{black!35}{0} & \textcolor{black!35}{0} & 18 & \textcolor{black!35}{0} & \textcolor{black!35}{0} & 24 \\
\addlinespace[2pt]
VAMOS & 0 & 30 & \textcolor{black!35}{0} & \textcolor{black!35}{0} & \textcolor{black!35}{0} & 1 & \textcolor{black!35}{0} & \textcolor{black!35}{0} & 25 & \textcolor{black!35}{0} & \textcolor{black!35}{0} & 26 \\
\addlinespace[2pt]
CityWalker + RL policy & 0 & 30 & 16 & \textcolor{black!35}{0} & \textcolor{black!35}{0} & 3 & \textcolor{black!35}{0} & \textcolor{black!35}{0} & \textcolor{black!35}{0} & \textcolor{black!35}{0} & \textcolor{black!35}{0} & 19 \\
CityWalker + RL policy & 2 & 30 & 10 & 2 & \textcolor{black!35}{0} & 4 & \textcolor{black!35}{0} & \textcolor{black!35}{0} & 2 & \textcolor{black!35}{0} & \textcolor{black!35}{0} & 18 \\
CityWalker + RL policy & 5 & 30 & 8 & 1 & \textcolor{black!35}{0} & 3 & 6 & 2 & 3 & 1 & \textcolor{black!35}{0} & 24 \\
CityWalker + RL policy & 7 & 30 & 4 & \textcolor{black!35}{0} & 1 & 4 & 9 & \textcolor{black!35}{0} & 5 & \textcolor{black!35}{0} & \textcolor{black!35}{0} & 23 \\
\addlinespace[2pt]
VAMOS + RL policy & 0 & 30 & 9 & 2 & \textcolor{black!35}{0} & \textcolor{black!35}{0} & \textcolor{black!35}{0} & \textcolor{black!35}{0} & \textcolor{black!35}{0} & \textcolor{black!35}{0} & \textcolor{black!35}{0} & 11 \\
VAMOS + RL policy & 2 & 30 & 11 & 1 & \textcolor{black!35}{0} & \textcolor{black!35}{0} & \textcolor{black!35}{0} & \textcolor{black!35}{0} & \textcolor{black!35}{0} & \textcolor{black!35}{0} & \textcolor{black!35}{0} & 12 \\
VAMOS + RL policy & 5 & 30 & 5 & 6 & 1 & 5 & 3 & 1 & 2 & 2 & \textcolor{black!35}{0} & 25 \\
VAMOS + RL policy & 7 & 30 & 2 & 3 & 2 & 7 & 6 & 1 & 2 & 4 & \textcolor{black!35}{0} & 27 \\
\addlinespace[2pt]
\method & 0 & 30 & \textcolor{black!35}{0} & \textcolor{black!35}{0} & 1 & \textcolor{black!35}{0} & \textcolor{black!35}{0} & 1 & \textcolor{black!35}{0} & 3 & \textcolor{black!35}{0} & 5 \\
\method & 2 & 30 & \textcolor{black!35}{0} & \textcolor{black!35}{0} & \textcolor{black!35}{0} & \textcolor{black!35}{0} & \textcolor{black!35}{0} & \textcolor{black!35}{0} & 1 & 5 & \textcolor{black!35}{0} & 6 \\
\method & 5 & 30 & 1 & \textcolor{black!35}{0} & \textcolor{black!35}{0} & 1 & \textcolor{black!35}{0} & \textcolor{black!35}{0} & 1 & 5 & \textcolor{black!35}{0} & 8 \\
\method & 7 & 30 & 1 & \textcolor{black!35}{0} & \textcolor{black!35}{0} & \textcolor{black!35}{0} & \textcolor{black!35}{0} & 1 & 1 & 8 & \textcolor{black!35}{0} & 11 \\
\addlinespace[2pt]
\method, oracle orchestrator & 0 & 30 & 2 & \textcolor{black!35}{0} & \textcolor{black!35}{0} & \textcolor{black!35}{0} & \textcolor{black!35}{0} & \textcolor{black!35}{0} & \textcolor{black!35}{0} & 1 & \textcolor{black!35}{0} & 3 \\
