# Supplementary material for: WayTrace: A Map-to-Language-to-Trace Hierarchy for Embodied Urban Navigation
Source: arXiv:2611.05129 source file (2026-11-03)
Supplement: Supplementary file 2 [file supp_missions.tex]

M1 & \anon{A}{Neumarkt} & Rheinfelder Bierhaus & 152 & 1 turn & 0 & 669 \\
M2 & \anon{B}{Bellevue} & Karl der Grosse & 223 & 1 turn & 0 & 858 \\
M3 & \anon{C}{Mühlesteg} & dieci pizza takeaway & 328 & 4 turns, 2 crossings & 2 & 1119 \\
M4 & \anon{C}{Mühlesteg} & Burger King & 361 & 2 turns, 3 crossings & 3 & 1195 \\
M5 & \anon{D}{Seilergraben} & Burger King & 393 & 1 fork, 2 crossings, stairs down & 3 & 1275 \\
M6 & \anon{D}{Seilergraben} & Café Zähringer & 406 & 2 crossings & 2 & 1308 \\
M7 & \anon{A}{Neumarkt} & Starbucks & 518 & 2 turns, 1 crossing & 1 & 1596 \\
M8 & \anon{B}{Bellevue} & Café Henrici & 633 & 1 turn & 0 & 1881 \\
M9 & \anon{E}{Zunfthaus zur Waag} & dieci pizza takeaway & 799 & 1 turn, 1 fork, 2 crossings & 2 & 2289 \\
M10 & \anon{F}{Limmatquai, Central} & Karl der Grosse & 864 & 2 turns, 2 crossings & 3 & 2461 \\
\midrule
\multicolumn{3}{l}{Total} & 4676 & 14 turns, 2 forks, 14 crossings, 1 staircase & 16 & \\
